# Supplementary material for: A pair of TESS planets spanning the radius valley around the nearby mid-M dwarf LTT 3780
Source: arXiv:2003.01136 source file (2020-05-12)
Supplement: Supplementary file 1 [file esmtable_tmp.tex]

\begin{tabular}{lrrrrrrrrrrr}
\toprule
{} &      P &     rp &         Z &          Teq &         Tday &    Kmag &    Teff &     Rs &     Ms &        ESM &   ESMnorm \\
\midrule
LTT 3780b   &  0.768 &  1.332 &  1.064354 &   892.852458 &   982.137704 &   8.204 &  3331.0 &  0.374 &  0.401 &  13.436062 &  0.463312 \\
LHS 3844b   &  0.463 &  1.303 &  3.988285 &   805.854400 &   886.439840 &   9.145 &  3036.0 &  0.189 &  0.151 &  29.000054 &  1.000002 \\
L 168-9b    &  1.402 &  1.390 &  0.450348 &   981.653764 &  1079.819140 &   7.082 &  3800.0 &  0.600 &  0.620 &   9.906946 &  0.341619 \\
GJ 1132b    &  1.629 &  1.130 &  2.406650 &   585.035999 &   643.539598 &   8.322 &  3270.0 &  0.211 &  0.181 &   9.537957 &  0.328895 \\
L 98-59b    &  2.250 &  0.800 &  0.558827 &   607.410761 &   668.151837 &   7.101 &  3412.0 &  0.310 &  0.310 &   4.127090 &  0.142313 \\
L 98-59c    &  3.690 &  1.350 &  1.591348 &   515.071909 &   566.579100 &   7.101 &  3412.0 &  0.310 &  0.310 &   6.858435 &  0.236498 \\
LTT 1445Ab  &  5.359 &  1.380 &  2.038276 &   435.075983 &   478.583582 &   6.500 &  3335.0 &  0.280 &  0.260 &   6.303129 &  0.217349 \\
TRAPPIST-1b &  1.511 &  1.090 &  6.923273 &   405.637555 &   446.201311 &  10.300 &  2559.0 &  0.120 &  0.080 &   3.974637 &  0.137056 \\
LHS 1140c   &  3.778 &  1.280 &  3.117470 &   434.050258 &   477.455284 &   8.821 &  3216.0 &  0.210 &  0.180 &   3.439983 &  0.118620 \\
LP 791-18b  &  0.948 &  1.120 &  3.599687 &   594.494693 &   653.944163 &  10.644 &  2949.0 &  0.171 &  0.139 &   5.912816 &  0.203890 \\
GJ 1252b    &  0.518 &  1.193 &  0.781175 &  1089.924342 &  1198.916776 &   7.915 &  3458.0 &  0.391 &  0.381 &  16.419351 &  0.566185 \\
\bottomrule
\end{tabular}
